# Supplementary material for: Bistable nanomagnet as programmable phase inverter for spin waves
Source: arXiv:2104.11015 ancillary file (2021-04-22)
Supplement: Supplementary file 1 [file Supplement_APL21-AR-MSFD2021-01725.pdf]

# Supplementary material to 'Bistable nanomagnet as programmable phase inverter for spin waves'

Korbinian Baumgaertl[1] and Dirk Grundler[1, 2, a)]

[1)] *Laboratory of Nanoscale Magnetic Materials and Magnonics, Institute of Materials (IMX), École Polytechnique Fédérale de Lausanne (EPFL), 1015 Lausanne, Switzerland*

[2)] *Institute of Microengineering (IMT), École Polytechnique Fédérale de Lausanne (EPFL), 1015 Lausanne, Switzerland*

(Dated: 9 April 2021)

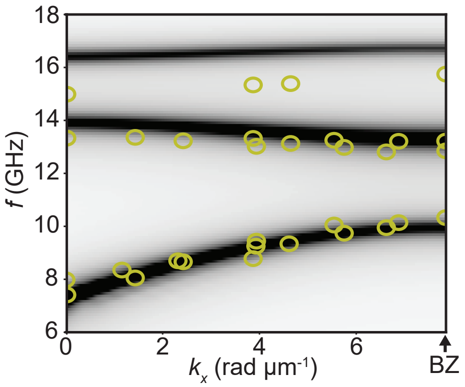


FIG. S1. Band structure of the simulated 1D MC (black branches) in comparison with the experimental band structure of MC1 (yellow dots)[1] shifted by $-1$ GHz. Simulation and experiment agree well for the first and second miniband. The frequency shift might be due to the approximation of the demagnetization tensor in the simulation using PBC in $y$-direction.

[a)] Electronic mail: dirk.grundler@epfl.ch

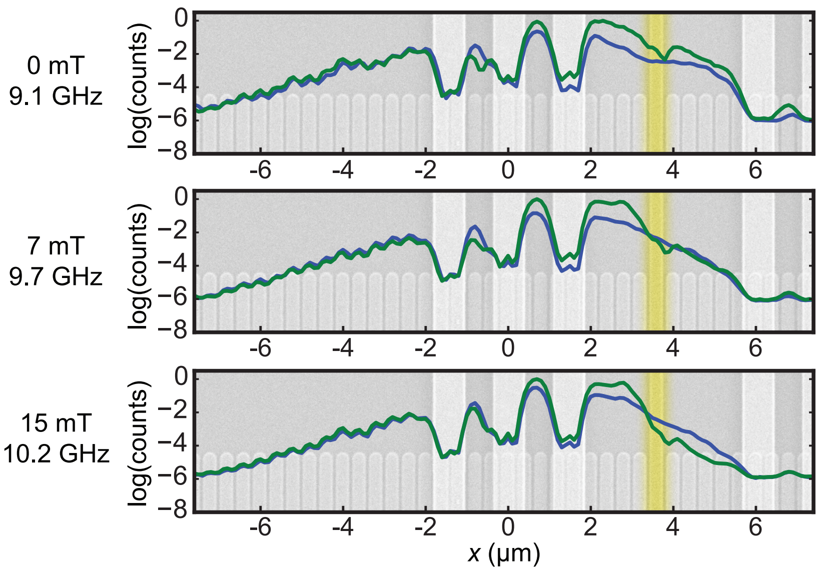


FIG. S2. SW intensity measured with (green lines) and without (blue lines) magnetic defect for different bias fields (rows). An aligned SEM image of MC1 is shown in the background of every plot as orientation. The position $x_\mathrm{D} = 3.6$ µm of the magnetic defect is highlighted in yellow. SWs on the left side of CPW1 followed an exponential decay. By fitting[2] in the region between $x = -7.6$ µm and $x = -2.1$ µm, we extract a decay length of $\delta = 2.9 \pm 0.2$ µm for $\mu_0 H = 0$ mT. SWs on the right side of CPW1 were modified by the presence of the magnetic defect. The amplitude attenuation ratio $\eta$ (in Fig. 2 of the main text) was calculated as square root of the ratio of BLS counts with defect to counts without defect extracted in the region from $x = 4.4$ µm to $x = 5.2$ µm. The square root was taken because BLS counts are proportional to $m_z^2$, while $\eta$ was defined as amplitude ratio. To correct for temporal drifts of the instrument's sensitivity, we extracted the amplitude ratio for $x < -2.1$ µm, i.e. for SWs which were unperturbed by the defect, and used this ratio as calibration factor for $\eta$.

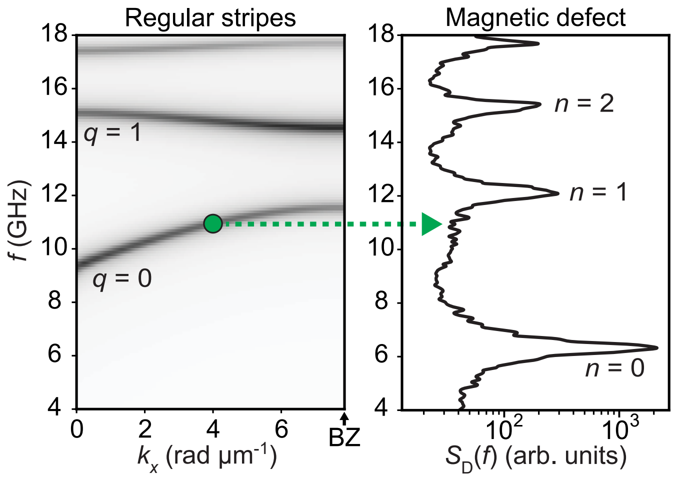


FIG. S3. Dispersion relation of the 1D MC and the power spectral density $S_\mathrm{D}(f)$ of thermally excited magnons at the defect simulated for $\mu_0 H = 24$ mT, respectively. At the frequency of SWs with 4 rad µm$^{-1}$ in the first miniband ($q = 0$) of the MC $S_\mathrm{D}(f)$ is low (see green arrow), indicating a forbidden frequency gap.

[1] K. Baumgaertl, S. Watanabe, and D. Grundler, Appl. Phys. Lett. **112**, 142405 (2018).
[2] T. Sebastian, Y. Ohdaira, T. Kubota, P. Pirro, T. Brächer, K. Vogt, A. A. Serga, H. Naganuma, M. Oogane, Y. Ando, and B. Hillebrands, Appl. Phys. Lett. **110**, 112402 (2012).
